# Supplementary material for: Contextual Active Model Selection
Source: arXiv:2207.06030 source file (2025-02-09)
Supplement: Supplementary file 1 [file supp_proofs_for_vc_dim.tex]

\clearpage
\section{Theoretical Results for Infinite Policy Class (Finite VC Dimension)}\label{sec:app:analysis:infinite}

Next, for learning from multiple policies problem, there is one challenge that the size of the policy class $|\Policies|$ could be extremely large or infinite. 
In this section, we focus on the adversarial setting, and consider infinite policy classes with a finite VC dimension.

Let us define the Vapnik-Chervnonenkis (VC) dimension of a hypothesis class $H$ as $\mathrm{VCdim}(H)$. $\mathrm{VCdim}(H)=\max{\paren{m\in N \mid \Pi_H\paren{m}=2^m}}$, which is the cardinality of the largest set of points in $X$ that can be shattered by hypothesis class $H$. We named the new algorithm $\algname_{\mathrm{VC}}$. Since it is in a standard VC-dimension definition, we assume we have only two base classifiers $\ModelsNum=2$. \citep{beygelzimer2011contextual} Here we only discussed the VC dimension for two actions/ classifiers. For multi-dimension, we could extend it by the Natarajan dimension.

We sketch our analysis framework below and provide the detailed analysis in the following subsections. $\algname_{\mathrm{VC}}$ first partitions the policy class $\Policies$ into equivalent classes based on each policy's sequential predictions at the first $\tau$ rounds. $\tau$ bounds the regret. Then it constructs a finite policy set $\Policies^{'}$ by picking a single policy from each class and testing \algname by using $\Policies^{'}$ on the rest $T-\tau$ rounds. By Sauer's lemma, we have $|\Policies^{'}|\leq \paren{\frac{e{\tau}}{d}}^d$. Combining it with \thmref{thm:adversarial-regret-bound},  we can get the regret bound of $\Loss_{\algname}\paren{\Policies^{'},T-\tau}$. Then we bound the regret of using policy set $\Policies^{'}$ to $\Policies$. We define the number of disagreement on the $T-\tau$ sequence as  $m = m\paren{\policy,\policy^{'}}$. Then we bound the agreement probability for size $\tau$ subset by $e^{-\frac{m\tau}{T}}$. Since there are $\paren{\frac{eT}{d}}^{2d}$ possible distinct pairs between $\Pi$ and $\Pi'$, we apply the union bound over every pair of policies. %
Finally, we reach the regret bound by combining the regret bounds from the above three parts.

\subsection{Regret bound} \label{app:vc_regret}
We formally state the regret bound for the infinite policy class setting as follows.

\begin{theorem}{(Regret)}\label{thm:vc-regret-bound}.
For any distributions over contexts and rewards, for all sets of policies $\Policies$ with VC dimension d, with probability $1-\frac{\delta}{2}$,
\[\mathcal{R}_T\paren{\algname}\leq
\paren{2|\domClabel|\sqrt{\ln{|\domClabel|}}+2}{{\sqrt{{T\cdot \paren{2d\ln{\frac{eT}{d}}+\ln{\frac{2}{\delta}}}}/{\fixremoved{\max}\{\minpgap{T},\fixremoved{\sqrt{1/T}}\}}}}}.
\]
\end{theorem}

The full proof for \thmref{thm:vc-regret-bound} 
is built upon \thmref{thm:adversarial-regret-bound}, while the proof structure depends on  \cite{beygelzimer2011contextual}.  %

\begin{proof}%

At the first $\tau$ rounds, the regret is bounded by $\tau$. In the following, we first bound the regret of \algname to policy set $\Policies^{'}$ for the remaining $T-\tau$ rounds, then we bound the regret of $\Policies^{'}$ to full policy set $\Policies$. 
In the end, we optimize with respect to the value of $\tau$ to achieve the result.

\emph{\underline{Step 1.} Bounding the regret of $\Loss_{\algname}\paren{\Policies^{'},T-\tau}:$}

Let us define $L_{\min}\paren{\Policies}$ as the return of the best policy in policy set $\Policies$ over T steps. By applying Sauer's lemma, we have $|\Policies^{'}|\leq \paren{\frac{e{\tau}}{d}}^d$, we can bound $\Loss_{\algname}\paren{\Policies^{'},T-\tau}$ with result from \thmref{thm:adversarial-regret-bound} by
\[
\Loss_{\algname}\paren{\Policies^{'},T-\tau} \leq \Loss_{\min{\paren{\Policies^{'}}}} + 2|\domClabel|\sqrt{\ln{|\domClabel|}}{\sqrt{\frac{\paren{T-\tau}\paren{d\ln{\frac{e\tau}{d}}}}{\fixremoved{\max}\{\minpgap{T-\tau},\fixremoved{\sqrt{1/{(T-\tau)}}}\}}}}.
\]

\emph{\underline{Step 2.} Bounding the regret of $\Policies^{'}$ to $\Policies:$ \\}
Sauer's Lemma implies the number of unique policies for any sequence of feature observations of context $x_1,...,x_T$ is bounded by $\paren{\frac{eT}{d}}^d$. Let us randomly pick subset $S$ of size $\tau$ of contexts and bound the probability that two policy $\pi$ and $\pi'$ agree on the subset. Let us defines the number of disagreement on the T-length sequence as $m = m\paren{\policy,\policy^{'}}$. Then

\[
\Prover{S}{\forall{x} \in S , \pi{\paren{x}}=\pi'{\paren{x}}}=\paren{1-\frac{m}{T}}^{\tau} \leq e^{-\frac{m\tau}{T}}\leq \delta_{0}
\]

Thus for any pair of $\policy,\policy' \in \Policies$ with $m\paren{\pi,\pi'}\geq \frac{T}{\tau}\ln{\frac{1}{\delta_{0}}}$, we 
have $Pr_S[\forall{x}\in S,\pi\paren{x}=\pi'\paren{x}]\leq \delta_{0}$. Since there are possible $\paren{\frac{eT}{d}}^{2d}$ distinct pairs between $\Pi$ and $\Pi'$.

We can get $\sum_{\Pi,\Pi'}\Pr{A\paren{\Pi,\Pi'}}\leq\paren{\frac{eT}{d}}^{2d}\delta_0$, 

\begin{flalign*}
\Pr{\bigcup_{\Pi,\Pi'}A\paren{\Pi,\Pi'}}\leq \sum_{\Pi,\Pi'}Pr\paren{A\paren{\Pi,\Pi'}} \leq\paren{\frac{eT}{d}}^{2d}\delta_0.
\end{flalign*}

Let us assume $\paren{\frac{eT}{d}}^{2d}\delta_0=\frac{\delta}{2}$, thus we get $\delta_0=\frac{\delta}{2}\paren{\frac{d}{eT}}^{2d}$. Since we have $m\paren{\pi,\pi'}\geq \frac{T}{\tau}\ln{\frac{1}{\delta_{0}}}$. 
By applying a union bound over every pair of policies, we get
\[
\Prover{S}{\exists \pi,\pi' , s.t. m\paren{\pi,\pi'} \geq \frac{T}{\tau}\paren{2d\ln\frac{eT}{d}+\ln{\frac{2}{\delta}}}}, 
\]
\[
s.t. {\forall{x}\in S,\pi\paren{x} = \pi'\paren{x}}\leq \frac{\delta}{2}.
\]

Hence, with probability $1-\frac{\delta}{2}$, we can get the following equation for any T-length sequences over a random subset of size $\tau$

\[
L_{\min}\paren{\Policies'}\leq L_{\min}\paren{\Policies} + \frac{T}{\tau}\paren{2d\ln\frac{eT}{d}+\ln{\frac{2}{\delta}}},
\]

Since the first $\tau$ samples of subset are from $i.i.d$ distribution and it is exchangeable. What's more, the above sequence holds for any T-length sequence. Consequently, with probability $1-\frac{\delta}{2}$, we have \\

\begin{flalign*}
\Loss_{\algname_{VC}} &\leq L_{\min}\paren{\Policies}+\tau +\frac{T}{\tau}\paren{2d\ln\frac{eT}{d}+\ln{\frac{2}{\delta}}} +2|\domClabel|\sqrt{\ln{|\domClabel|}}{\sqrt{\frac{\paren{T-\tau}\paren{d\ln{\frac{e\tau}{d}}}}{{\fixremoved{\max}\{\minpgap{T-\tau},\fixremoved{\sqrt{1/{(T-\tau)}}}\}}}}}\\
&\leq L_{\min}\paren{\Policies} +\tau +\frac{T}{\tau{\fixremoved{\max}\{\minpgap{T},\fixremoved{\sqrt{1/{T}}}\}}}\paren{2d\ln\frac{eT}{d}+\ln{\frac{2}{\delta}}} +2|\domClabel|\sqrt{\ln{|\domClabel|}}{\sqrt{\frac{T\cdot \paren{2d\ln{\frac{eT}{d}}+\ln{\frac{2}{\delta}}}}{{\fixremoved{\max}\{\minpgap{T},\fixremoved{\sqrt{1/{T}}}\}}}}}.
\end{flalign*}

\emph{\underline{Step 3.} Optimizing over $\tau$.} 

Let $\tau = {\sqrt{\frac{T\cdot \paren{2d\ln{\frac{eT}{d}}+\ln{\frac{2}{\delta}}}}{{\fixremoved{\max}\{\minpgap{T},\fixremoved{\sqrt{1/{T}}}\}}}}}$. We get

\begin{align*}
\Loss_{\algname_{\mathrm{VC}}} &\leq L_{\min}\paren{\Policies} + \paren{2|\domClabel|\sqrt{\ln{|\domClabel|}}+2}{{\sqrt{\frac{T\cdot \paren{2d\ln{\frac{eT}{d}}+\ln{\frac{2}{\delta}}}}{{\fixremoved{\max}\{\minpgap{T},\fixremoved{\sqrt{1/{T}}}\}}}}}}\\
&\stackrel{\paren{a}}{\leq} \tilde{\Loss}_{T,*} + \paren{2|\domClabel|\sqrt{\ln{|\domClabel|}}+2}{{\sqrt{\frac{T\cdot \paren{2d\ln{\frac{eT}{d}}+\ln{\frac{2}{\delta}}}}{{\fixremoved{\max}\{\minpgap{T},\fixremoved{\sqrt{1/{T}}}\}}}}}},
\end{align*}
where step (a) is by replacing $L_{\min}\paren{\Policies}= \tilde{\Loss}_{T,*}$.

\end{proof}

\subsection{Query complexity bound} 
\label{app:vc_query_complexity}

By following the proof of \thmref{thm:stochastic-query-complexity} and adapting the regret bound of \thmref{thm:vc-regret-bound}, we prove the sub-linear query complexity for the infinite policy class setting as follows. %
\begin{theorem}{(Query Complexity, informal)}\label{thm:vc-query-complexity}. Assume at least two models disagree at each round in a $|\domClabel|$ classification problem and assume for all sets of policies $\Policies$ with VC dimension $d$. For T $\geq$ 0, the expected query number till round T under VC Dimension setting with probability $1-\delta$ is at most
\[
{O}\paren{
\frac{{\ln\paren{T}}}{|\domClabel|\ln{|\domClabel|}}\paren{{{\sqrt{\frac{T\cdot \paren{2d\ln{\frac{eT}{d}}+\ln{\frac{2}{\delta}}}}{\fixremoved{\max}\{\minpgap{T},\fixremoved{\sqrt{1/T}}\}}}}}+\tilde{\Loss}_{T,*}}}.
\]
\end{theorem}

\begin{proof}%
From \lemref{lem:query_complexity}, we get the following equation as the cumulative query cost
\[
\expct{\sum_{t=1}^TU_t} \leq
\expct{\sum_{t=1}^T{\paren{\frac{1}{\sqrt{t}}+\frac{\sum_{y\in \domClabel} \langle \ModelsDistB_t,\lossB_t^y \rangle \log_{|\domClabel|}{\frac{1}{\langle \ModelsDistB_t,\lossB_t^y \rangle}}}{|\domClabel|}}}}.
\]

Let us assume the expected total loss of best policy is $\tilde{\Loss}_{T,*}$, thus from $\thmref{thm:vc-regret-bound}$, we get 

\[
    \expct{R_T}=\expct{\sum_{t=1}^T r_t}\leq \paren{2|\domClabel|\sqrt{\ln{|\domClabel|}}+2}{{\sqrt{\frac{T\cdot \paren{2d\ln{\frac{eT}{d}}+\ln{\frac{2}{\delta}}}}{{\fixremoved{\max}\{\minpgap{T},\fixremoved{\sqrt{1/{T}}}\}}}}}} + \tilde{\Loss}_{T,*}.
\]

By using \eqnref{eq:budget-eq}, we can get the following query complexity theory.
\begin{flalign*}
\expct{\sum_{t=1}^TU_t}&\leq 2\sqrt{T}+\\
&\frac{\paren{ \paren{2|\domClabel|\sqrt{\ln{|\domClabel|}}+2}{{\sqrt{\frac{T\cdot \paren{2d\ln{\frac{eT}{d}}+\ln{\frac{2}{\delta}}}}{{\fixremoved{\max}\{\minpgap{T},\fixremoved{\sqrt{1/{T}}}\}}}}}}+\tilde{\Loss}_{T,*}}\paren{\log_{|\domClabel|}\frac{T^2\paren{|\domClabel|-1}}{\paren{ \paren{2|\domClabel|\sqrt{\ln{|\domClabel|}}+1}{{\sqrt{\frac{T\cdot \paren{2d\ln{\frac{eT}{d}}+\ln{\frac{2}{\delta}}}}{{\fixremoved{\max}\{\minpgap{T},\fixremoved{\sqrt{1/{T}}}\}}}}}}+\tilde{\Loss}_{T,*}}^2}}}{|\domClabel|}\\
&\leq 2\sqrt{T}+\frac{\paren{\paren{2|\domClabel|\sqrt{\ln{|\domClabel|}}+2}{{\sqrt{\frac{T\cdot \paren{2d\ln{\frac{eT}{d}}+\ln{\frac{2}{\delta}}}}{{\fixremoved{\max}\{\minpgap{T},\fixremoved{\sqrt{1/{T}}}\}}}}}}+\tilde{\Loss}_{T,*}}\paren{\log_{|\domClabel|}{\paren{T|\domClabel|}}}}{|\domClabel|},\\
\end{flalign*}

since the second term dominates the upper bound, we have
\begin{align*}
{O}\paren{\expct{\sum_{t=1}^TU_t}}&={O}\paren{
\frac{\paren{{{\sqrt{\frac{T\cdot \paren{2d\ln{\frac{eT}{d}}+\ln{\frac{2}{\delta}}}}{{\fixremoved{\max}\{\minpgap{T},\fixremoved{\sqrt{1/{T}}}\}}}}}}+\tilde{\Loss}_{T,*}}\paren{\ln\paren{T}}}{|\domClabel|\ln{|\domClabel|}}}\\
&\stackrel{\paren{a}}{=}\fixremoved{{O}\paren{
\frac{\paren{{{\sqrt{\frac{T\cdot \paren{2d\ln{\frac{eT}{d}}+\ln{\frac{2}{\delta}}}}{{\fixremoved{\max}\{\minpgap{T},\fixremoved{\sqrt{1/{T}}}\}}}}}}+\tilde{\Loss}_{T,*}}\paren{\ln\paren{T}}}{\numClabel\ln{\numClabel}}},}
\end{align*}

\fixremoved{where step (a) is by applying $\numClabel=|\domClabel|$.}

\end{proof}
