# Supplementary material for: Contextual Active Model Selection
Source: arXiv:2207.06030 source file (2025-02-09)
Supplement: Supplementary file 2 [file appendix.tex]

\addcontentsline{toc}{section}{Appendix} %

\parttoc %

\vfill

\clearpage
