# Supplementary material for: Contextual Active Model Selection
Source: arXiv:2207.06030 source file (2025-02-09)
Supplement: Supplementary file 4 [file supp_miscellaneous.tex]

\clearpage
\section{\fix{Miscellaneous}}

\subsection{How tight is the bound for query complexity in practice?}
We observe (in \figref{fig:exp:results}, Middle plots) that the query complexity grows sublinear in $T$. Although we do not have tightness results of the query complexity bounds, the proofs of  \thmref{thm:stochastic-query-complexity} and \thmref{thm:adversarial-query-complexity} are built on top of the regret bounds. In our revision, we have added to 
\secref{sec:analysis} (Theoretical Analysis) that our regret bounds in both stochastic settings and adversarial settings are tight up to a constant factor of existing lower bounds. We acknowledge that it is non-trivial to come up with a query complexity lower bound, and leave it as an interesting direction for future work.
